# Supplementary material for: Interactive Image Restoration
Source: arXiv:1910.11059 source file (2019-10-24)
Supplement: Supplementary file 1 [file Statistics.pdf]

# Survey - Image Reconstruction

21 responses

Data Protection

## Expertise

### Please answer how you agree with the following statements

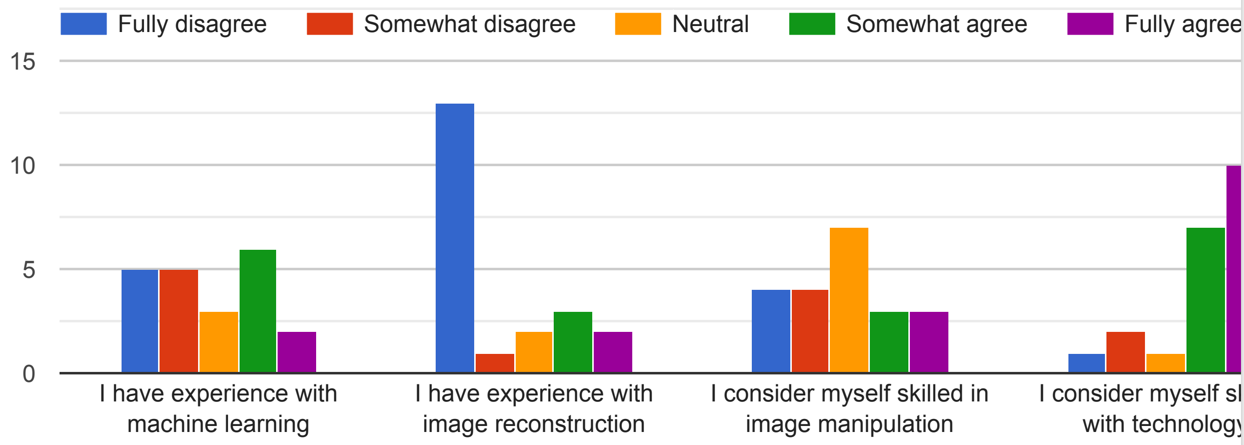


## Machine Learning Support

### Please answer how you agree with the following statements

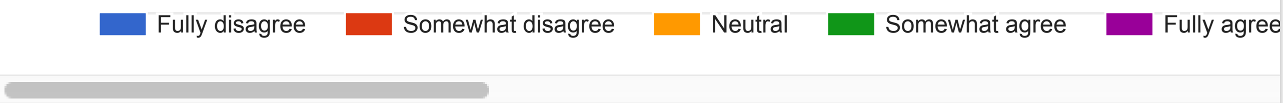


## Please answer how you agree with the following statements

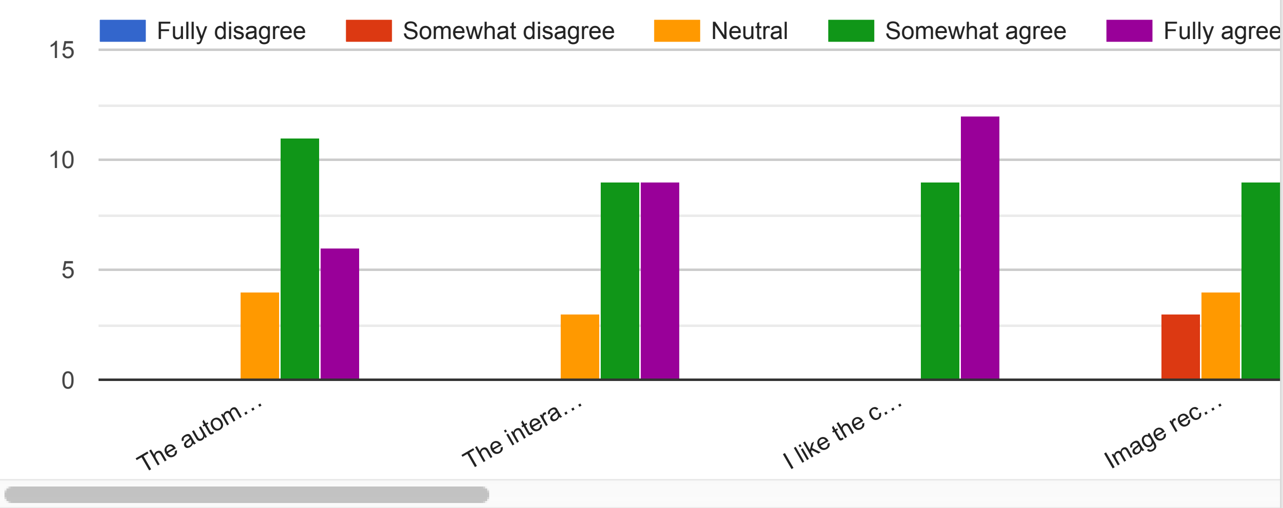


## Did anything during the task not work the way you would have wanted it to?

8 responses

No

Sometimes the pen tool gets automatically deselected when switching between pipette and pen.

I thought that the algorithm could also reconstruct sharp edges but it didn't.

No, everything worked well

when you moved the mouse outside the image while painting on the edges it continued drawing

I would like to use the pen firstly draw a boundary, and fullfil it with the coulor. The ColorPicker is sometime not sensitive enough to pick up the small area color.

## What would you change in the interactive image reconstruction process?

11 responses

Let the automated process run in parallel and in background, so you have to wait less.

comparing some images with similar ones (pattern recognition, duplicated elements,...)

maybe more professional drawing brushes that I can give more details.

size of the tool could be symbolized

Shorter processing time.

for now nothing

Nothing

Introduce instructions by voice

Adding zoom functions.

The mouse for a finer pencil-like item

Copy patch instead of only one color

# General System Usability

## Please answer how you agree with the following statements

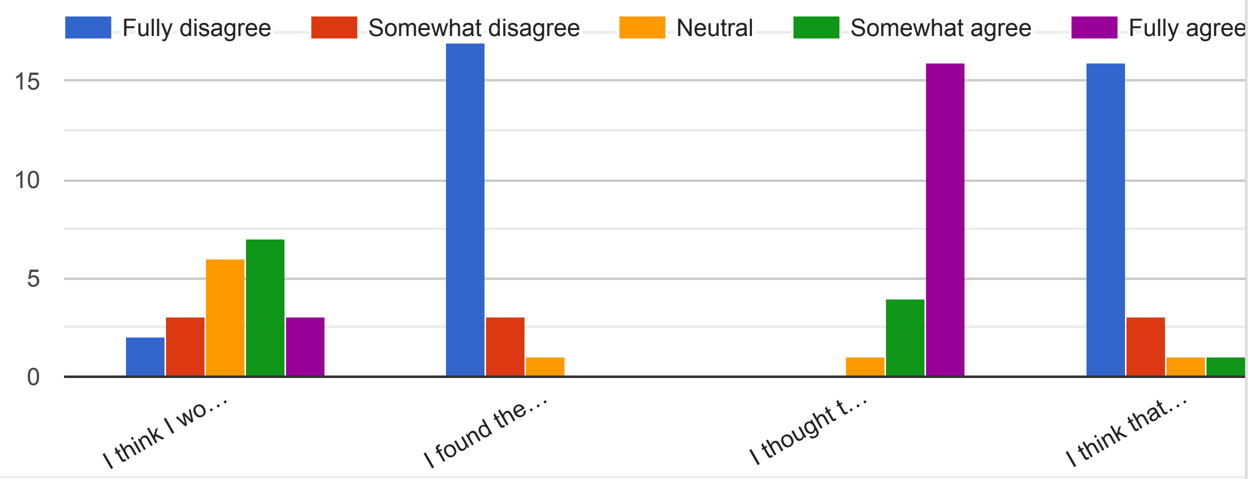

## Workload

### How mentally demanding was the task?

21 responses

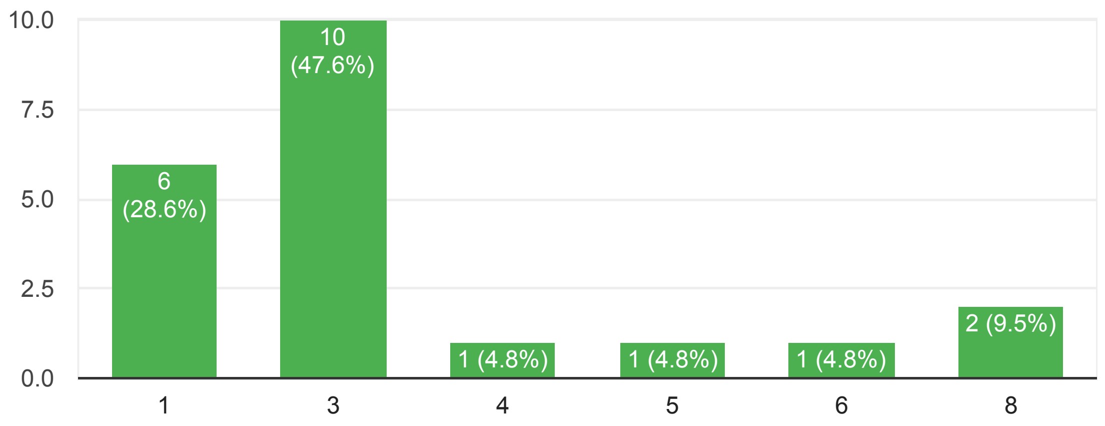


### How physically demanding was the task?

21 responses

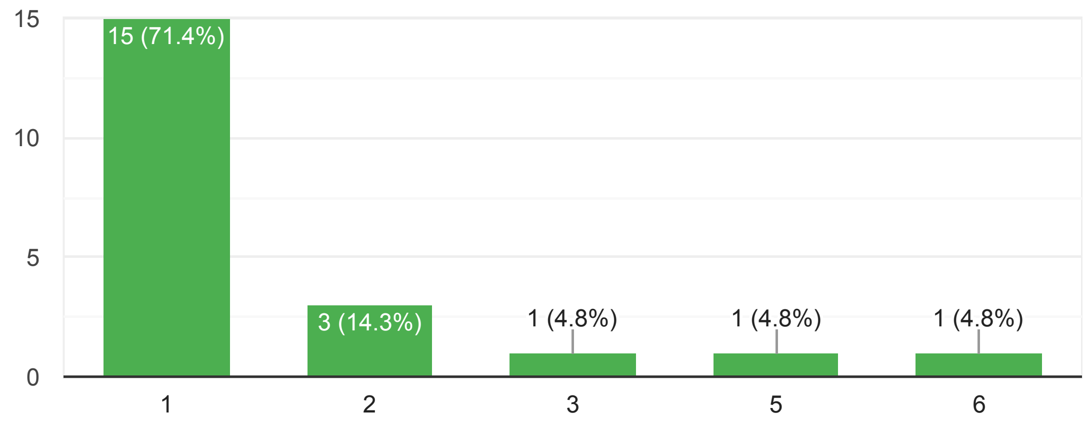


### How hurried or rushed was the pace of the task?

21 responses

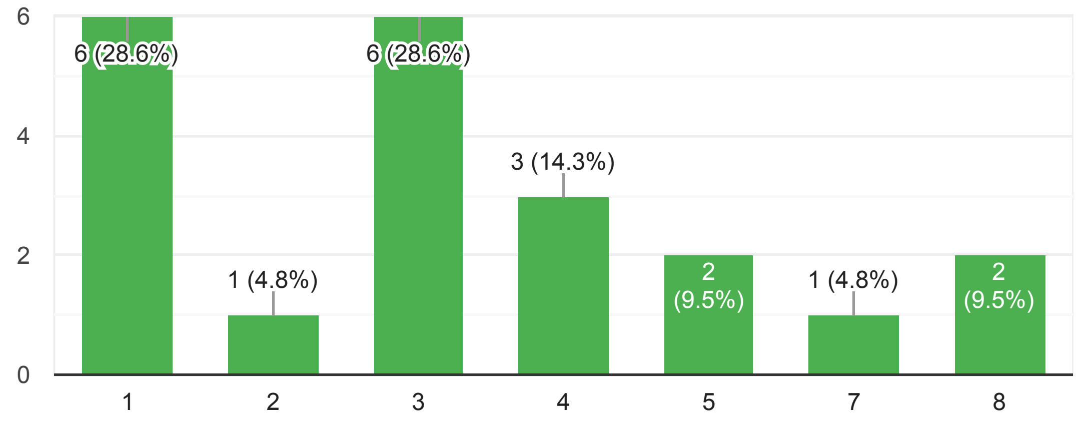


## How successful were you in accomplishing what you were asked to do?

21 responses

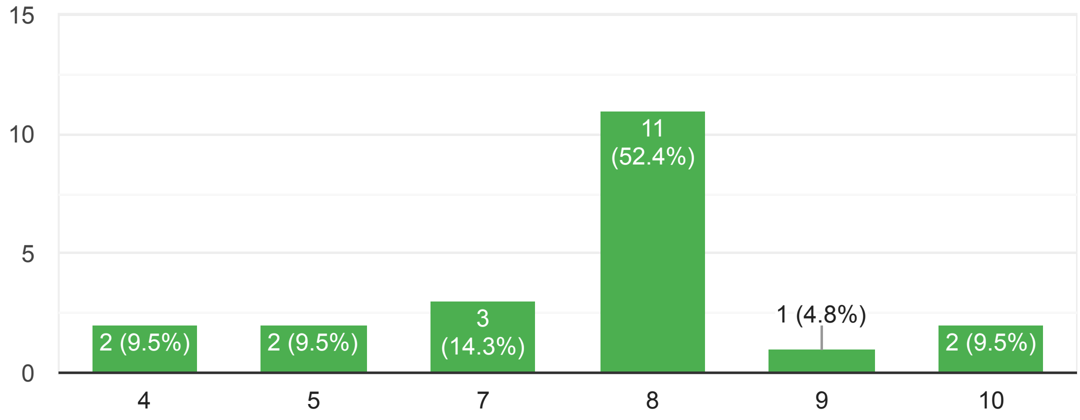


## How hard did you have to work to accomplish your level of performance?

21 responses

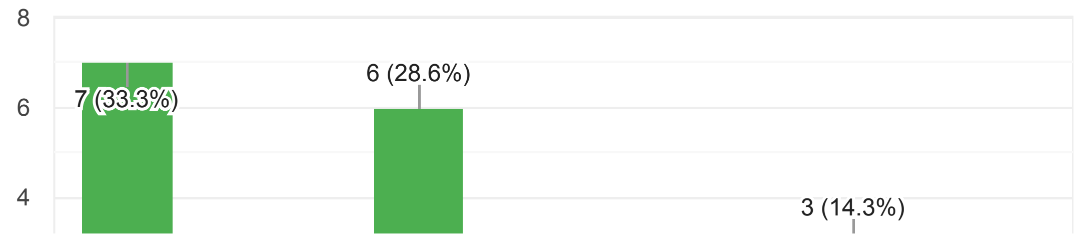


## How insecure, discourage, irritated, stressed and annoyed were you?

21 responses

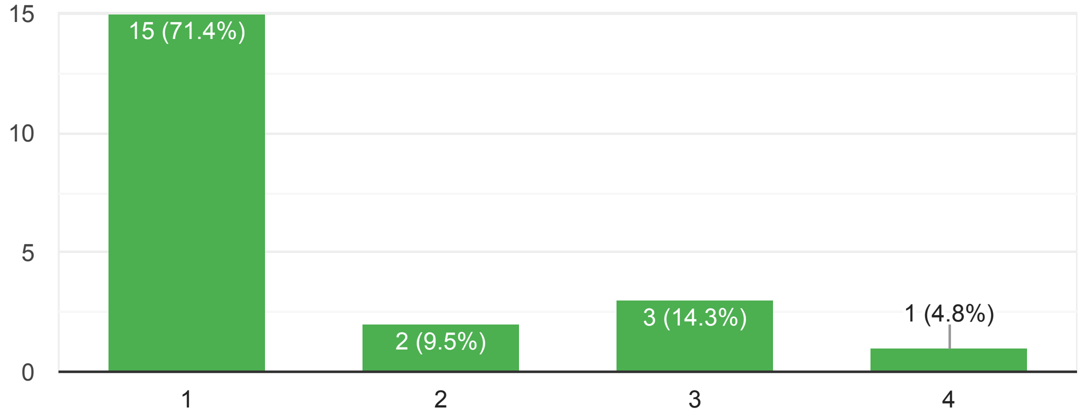


## Demographics

## How old are you?

21 responses

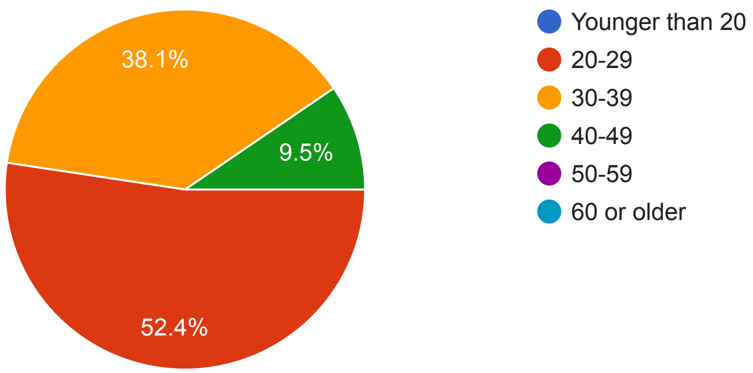

## What is your gender?

21 responses

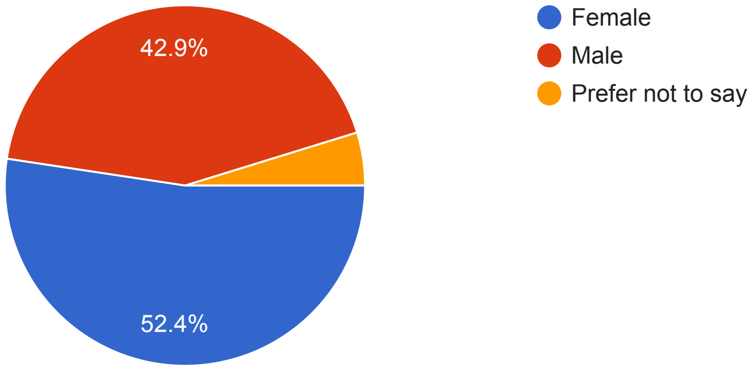


This content is neither created nor endorsed by Google. Report Abuse - Terms of Service

Google Forms
