# Supplementary material for: Interactive Image Restoration
Source: arXiv:1910.11059 source file (2019-10-24)
Supplement: Supplementary file 2 [file Survey.pdf]

1. **Please answer how you agree with the following statements** *

*Mark only one oval per row.*

| | Fully disagree | Somewhat disagree | Neutral | Somewhat agree | Fully agree |
|---|---|---|---|---|---|
| I can draw | ◯ | ◯ | ◯ | ◯ | ◯ |
| I have experience with machine learning | ◯ | ◯ | ◯ | ◯ | ◯ |
| I consider myself skilled in image manipulation | ◯ | ◯ | ◯ | ◯ | ◯ |
| I have previous experience with image manipulation software | ◯ | ◯ | ◯ | ◯ | ◯ |
| I consider myself skilled with technology | ◯ | ◯ | ◯ | ◯ | ◯ |
| I am open towards new technology | ◯ | ◯ | ◯ | ◯ | ◯ |
| I have experience with image reconstruction | ◯ | ◯ | ◯ | ◯ | ◯ |

# Machine Learning Support

In the following section you will answer some questions regarding the task you have performed and the tool you have used.

2. **Please answer how you agree with the following statements** *

*Mark only one oval per row.*

| | Fully disagree | Somewhat disagree | Neutral | Somewhat agree | Fully agree |
|---|---|---|---|---|---|
| A human can perform Image reconstruction better than a machine | ◯ | ◯ | ◯ | ◯ | ◯ |
| Tools using machine learning are more efficient | ◯ | ◯ | ◯ | ◯ | ◯ |
| Machine learning should only be used where necessary | ◯ | ◯ | ◯ | ◯ | ◯ |
| Tools using machine learning are more effective | ◯ | ◯ | ◯ | ◯ | ◯ |
| Machine learning is a good support mechanism in tools | ◯ | ◯ | ◯ | ◯ | ◯ |
| I want more machine learning support in tools | ◯ | ◯ | ◯ | ◯ | ◯ |
| Machine learning is helpful for image reconstruction | ◯ | ◯ | ◯ | ◯ | ◯ |
| Machine learning should be used more frequently | ◯ | ◯ | ◯ | ◯ | ◯ |
| Tools using machine learning help me complete my work faster | ◯ | ◯ | ◯ | ◯ | ◯ |
| Machine learning takes a long time | ◯ | ◯ | ◯ | ◯ | ◯ |

3. **Please answer how you agree with the following statements** *

*Mark only one oval per row.*

| | Fully disagree | Somewhat disagree | Neutral | Somewhat agree | Fully agree |
|---|---|---|---|---|---|
| I like the combination of interactive and automated elements for image reconstruction | ⬭ | ⬭ | ⬭ | ⬭ | ⬭ |
| I am satisfied with the result | ⬭ | ⬭ | ⬭ | ⬭ | ⬭ |
| I was in control of how the output turned out | ⬭ | ⬭ | ⬭ | ⬭ | ⬭ |
| Image reconstruction should be more automated | ⬭ | ⬭ | ⬭ | ⬭ | ⬭ |
| The interactive part of the image reconstruction worked well | ⬭ | ⬭ | ⬭ | ⬭ | ⬭ |
| The image turned out the way I expected it to | ⬭ | ⬭ | ⬭ | ⬭ | ⬭ |
| The automated part of the image reconstruction worked well | ⬭ | ⬭ | ⬭ | ⬭ | ⬭ |
| Machine learning without interactivity would create a better image | ⬭ | ⬭ | ⬭ | ⬭ | ⬭ |
| Manual image reconstruction would create a better image | ⬭ | ⬭ | ⬭ | ⬭ | ⬭ |
| Image reconstruction should be done manually | ⬭ | ⬭ | ⬭ | ⬭ | ⬭ |

4. **Did anything during the task not work the way you would have wanted it to?**

_______________________________________________
_______________________________________________
_______________________________________________
_______________________________________________
_______________________________________________

5. **What would you change in the interactive image reconstruction process?**

_______________________________________________
_______________________________________________
_______________________________________________
_______________________________________________
_______________________________________________

## General System Usability

In the following section you will answer some questions regarding the usability of the system we have presented to you.

6. **Please answer how you agree with the following statements** *
*Mark only one oval per row.*

| | Fully disagree | Somewhat disagree | Neutral | Somewhat agree | Fully agree |
|---|---|---|---|---|---|
| I need to learn a lot of things before I could get going with the system | ⬭ | ⬭ | ⬭ | ⬭ | ⬭ |
| I found the system very cumbersome to use | ⬭ | ⬭ | ⬭ | ⬭ | ⬭ |
| I felt very confident using the system | ⬭ | ⬭ | ⬭ | ⬭ | ⬭ |
| I thought there was too much inconsistency in this system | ⬭ | ⬭ | ⬭ | ⬭ | ⬭ |
| I think I would like to use this system frequently | ⬭ | ⬭ | ⬭ | ⬭ | ⬭ |
| I found the system unnecessarily complex | ⬭ | ⬭ | ⬭ | ⬭ | ⬭ |
| I found the various functions in the system well integrated | ⬭ | ⬭ | ⬭ | ⬭ | ⬭ |
| I would imagine that most people would learn to use this system very quickly | ⬭ | ⬭ | ⬭ | ⬭ | ⬭ |
| I thought the system was easy to use | ⬭ | ⬭ | ⬭ | ⬭ | ⬭ |
| I think that I would need support of a technical person to be able to use the system | ⬭ | ⬭ | ⬭ | ⬭ | ⬭ |

# Workload

In the following section you will answer some questions on the perceived workload for the task.
You can give a score from 1 to 10 where 1 means "low" or "not much" while 10 means "high" or "a lot".

7. **How mentally demanding was the task?**

______________________________

8. **How physically demanding was the task?**

______________________________

9. **How hurried or rushed was the pace of the task?**

______________________________

10. **How successful were you in accomplishing what you were asked to do?**

______________________________

11. **How hard did you have to work to accomplish your level of performance?**

______________________________

12. **How insecure, discourage, irritated, stressed and annoyed were you?**

______________________________

# Demographics

Lastly we ask you for some general information about yourself

13. **How old are you?**

*Mark only one oval.*

- Younger than 20
- 20-29
- 30-39
- 40-49
- 50-59
- 60 or older

14. **What is your gender?**

*Mark only one oval.*

- Female
- Male
- Prefer not to say
- Other: ____________________

Powered by
Google Forms
